# Supplementary material for: Non-Contrastive Learning-based Behavioural Biometrics for Smart IoT Devices
Source: arXiv:2210.12964 source file (2022-10-24)
Supplement: Supplementary file 1 [file Appendix.tex]

\section{Appendix}
\label{Sec:appendix}

\begin{table*}[h]
\centering
\smaller
\begin{tabular}{p{1.5cm}p{7cm}}
\toprule
\textbf{Scenario} & \textbf{Research Question}\\\hline\hline
1 & Can non-contrastive SSL be used to leverage unlabelled data from a set of users to build a label-efficient classifier for a completely different set of users?\\ \hline
2 & Can non-contrastive SSL be used to leverage unlabelled data from a given set of user to train a label-efficient classifier for user authentication?\\ \hline
3 & Can non-contrastive SSL be used to leverage unlabelled data
from a initial set of users to build a label-efficient classifier for both initial set of users and a whole new set of users?
\\\bottomrule
\end{tabular}
\caption{Summary of research questions and baselines}
\label{tab:baselines}
\end{table*}
